# Supplementary material for: FedAFD: Multimodal Federated Learning via Adversarial Fusion and Distillation
Source: arXiv:2603.04890 source file (2026-03-05)
Supplement: Supplementary file 1 [file X_new_suppl.tex]

\clearpage
\setcounter{page}{1}
\maketitlesupplementary
\appendix
\section{Algorithm and Implementation Details}
\subsection{Algorithm Training Framework}
FedAFD consists of two alternate steps, \textit{i.e.}, distributed local training and centralized server update.

\subsubsection{Local Training Step}\label{sec:LearnLocal}
Taking image clients as an example, clients update the local model $w_{c}$, consisting of the feature extractor $\phi_c$, intra-modal discriminator $\mathcal{D}_c^{in}$, cross-modal discriminator $\mathcal{D}_c^{cr}$, GFF module $\mathcal{A}_c$, and local classification $\mathcal{C}_c$, by solving the following function:
\begin{equation}
\begin{aligned}
&(\mathcal{D}_c^{in*},\mathcal{D}_c^{cr*})= \arg \mathop {\max{\rm{ }}}\limits_{\mathcal{D}_c^{in},\mathcal{D}_c^{cr}}(\mathcal{L}_{adv}),\\
&(\mathcal{A}_c^*,\mathcal{C}_c^*) = 
\arg\mathop {\min{\rm{ }}}\limits_{\mathcal{A}_c, \mathcal{C}_c}(\mathcal{L}_{task}),\\
&(\phi_c^*)= \arg\mathop {\min{\rm{ }}}\limits_{\mathcal\phi_c}(\mathcal{L}_{task}+\beta\cdot\mathcal{L}_{adv}),\\
% &(\mathcal{D}_c^{in*},\mathcal{D}_c^{cr*},\phi_c^*)= \arg \mathop{\min}\limits_{\phi_c}\mathop {\max{\rm{ }}}\limits_{\mathcal{D}_c^{in},\mathcal{D}_c^{cr}}(\mathcal{L}_{adv}),\\
% &(\mathcal{A}_c^*,\mathcal{C}_c^*,\phi_c^*) = 
% \mathop {\arg\min{\rm{ }}}\limits_{\mathcal{A}_c, \mathcal{C}_c, \phi_c}(\mathcal{L}_{t} + \beta \mathcal{L}_{adv}),\\
% &(\mathcal{D}_c^{in*},\mathcal{D}_c^{cr*},\phi_c^*, A_c^*,C_c^*) = 
% \arg \mathop{\min}\limits_{\phi_c, A_c, C_c} \mathop{\max}\limits_{\mathcal{D}_c^{in}, \mathcal{D}_c^{cr}} (\mathcal{L}_{t} + \beta \mathcal{L}_{adv}),\\
% &(\mathcal{D}_c^{in*},\mathcal{D}_c^{cr*})= \mathop {\arg\min{\rm{ }}}\limits_{\mathcal{D}_c^{in},\mathcal{D}_c^{cr}}(\mathcal{L}_{adv}),\\
% &(A_c^*,C_c^*)= \mathop {\arg\min{\rm{ }}}\limits_{A_c,C_c}\mathcal{L}_{t},\\
% &(\phi_c^*)= \mathop {\arg\min{\rm{ }}}\limits_{\mathcal\phi_c}(\mathcal{L}_{t}-\beta\cdot\mathcal{L}_{adv}),\\
&s.t.\;\left\{ \begin{array}{l}
\mathcal{L}_{task}=\frac{1}{|\mathcal{I}_c|}\sum_{k=1}^{|\mathcal{I}_c|}l(\widetilde{i}_c^k,y_c^k;w_c),\\
\mathcal{L}_{adv}=\frac{1}{|\mathcal{P}|}\sum_{k=1}^{|\mathcal{P}|}(\mathcal{L}_{\text{in}}^{k}+\mathcal{L}_{\text{cr}}^{k}),\\
\widetilde{i}_c^k = \mathcal{A}_c(i_c^k,i_g^k),
\end{array} \right.
\end{aligned}
\label{eq:localtrain}
\end{equation}
where $\beta$ is a tradeoff hyperparameter. Note that, in Eq.(\ref{eq:localtrain}), the task loss $\mathcal{L}_{t}$ is computed on the fused feature $\widetilde{i}_c^k$.

\subsubsection{Centralized Training Step}
The global model is updated in two stages. In the first stage, we optimize the global model on public data using a standard task-specific loss function:
\begin{equation}
\begin{aligned}
w_g := w_g - \eta \nabla \mathcal{L}(\mathcal{P}; w_g^t),
\end{aligned}
\end{equation}
where $l(\cdot)$ is task-specific loss computed on public dataset, $\eta$ is the learning rate, and $\nabla$ denotes the gradient operator.

Afterwards, we leverage the representations generated by the heterogeneous local models to further enhance the global model via ensemble distillation. The corresponding update rule for this stage is given by:
\begin{equation} 
\begin{aligned}
w_g := w_g - \eta\cdot\gamma \nabla \mathcal{L}_{kd},
\end{aligned}
\label{eq:kd}
\end{equation}
where $\gamma$ is a balancing coefficient. %that controls the influence of the distillation loss.
\subsection{Network Architecture Specifications}
\subsubsection{Discriminator Networks in BAA}
Each adversarial discriminator $\mathcal{D}$ in the Bi-level Adversarial Alignment (BAA) module is implemented as a binary classification network. Its objective is to distinguish between feature vectors originating from the client's local distribution and those from the server's global distribution.

The discriminator $\mathcal{D}:\mathbb{R}^d \rightarrow [0,1]$ is a multilayer perceptron composed of the following sequence of layers:\\
1. A linear layer that maps the input feature of dimension $d=256$ to a hidden dimension of 128.\\
2. A LeakyReLU activation with a negative slope of 0.2.\\
3. A linear layer that maps from 128 to 64 dimensions.\\
4. Another LeakyReLU activation with a slope of 0.2.\\
5. A final linear layer that projects the 64-dimensional hidden representation to a single scalar.\\
6. A Sigmoid activation function that squashes the output into a range [0,1], interpreted as the probability that the input feature comes from the server's global distribution.
\subsubsection{Attention Network in GFF}
The transformations are implemented as:
\begin{equation}
    T_1(x) = \text{B}(\text{Conv}_{2}( \sigma(\text{B}(\text{Conv}_{1}(\text{GAP}(x)))))),
\end{equation}
\begin{equation}
    T_2(x) = \text{B}(\text{Conv}_{2}( \sigma(\text{B}(\text{Conv}_{1}(x))))),
\end{equation}
where $\text{Conv}$ denotes point-wise convolutional layers, $\text{B}$ denotes batch normalization and $\text{GAP}$ denotes to global average pooling.

\section{Additional Theoretical Analysis}
\begin{table*}
\centering
\begin{tabular*}{\hsize}{@{}@{\extracolsep{\fill}}lccc cc c c@{}}
\toprule
\multirow{3}{*}
{Method}&\multicolumn{4}{c}{Clients}&\multicolumn{3}{c}{Server}
\\\cline{2-5} \cline{6-8}&CIFAR-100&AGNEWS&\multicolumn{2}{c}{Flickr30k}&\multicolumn{3}{c}{MS-COCO}\\
\cline{2-2} \cline{3-3} \cline{4-5} \cline{6-8}
&acc@1&acc@1&i2t R@1&t2i R@1&i2t R@1&t2i R@1&rsum R@1\\
\hline
LOCAL&28.07&48.35&22.33&18.44&32.48&25.06&57.54\\
\midrule
FedMD&22.54&48.18&19.13&15.63&33.00&25.47&58.47\\
FedGEMS&22.84&48.30&18.93&16.05&33.12&25.50&58.62\\
FedET&31.86&49.38&22.63&18.22&33.20&25.72&58.92\\
CreamFL&22.14&42.16&18.38&15.49&33.72&25.89&59.61\\
FedMKD&24.99&47.99&22.33&18.37&33.24&25.94&59.18\\
FedDFA&23.09&43.79&19.68&17.13&33.56&25.54&59.10\\
\midrule
FedAFD&33.18&51.98&32.48&25.68&33.98&26.18&60.16\\
FedAFD($K$=10)&32.91&51.40&30.63&24.09&33.76&26.12&59.88\\
\bottomrule
\end{tabular*}
\caption{Performance comparison with baselines on diverse clients and the server under Non-IID settings.}
\label{K}
\end{table*}

\begin{table}
\centering
\begin{tabular}{lccc}
\toprule
Method&Upload&Download&Sum\\
\hline
FedMD&19.54MB&19.54MB&39.08MB\\
FedGEMS&19.54MB&19.54MB&39.08MB\\
FedET&51.80MB&51.80MB&103.60MB\\
CreamFL&19.54MB&19.54MB&39.08MB\\
FedMKD&19.54MB&19.54MB&39.08MB\\
FedDFA&19.54MB&19.54MB&39.08MB\\
\midrule
FedAFD&19.54MB&49.26MB&68.80MB\\
% FedAFD&19.54MB&316.70MB&336.24MB\\
\bottomrule
\end{tabular}
\caption{Comparison of communication cost.}
\label{communication cost}
\end{table}

\begin{table}
\centering
\begin{tabular}{lc}
\toprule
Method&Time(seconds)\\
\hline
FedMD&959\\
FedGEMS&974\\
FedET&503\\
CreamFL&975\\
FedMKD&498\\
FedDFA&954\\
\midrule
FedAFD&1034\\
\bottomrule
\end{tabular}
\caption{Average Training Time per Round.}
\label{Computational cost}
\end{table}

\begin{table}[t]
\centering
\footnotesize
\label{tab:client_cost}
\begin{tabular}{ccc}
\toprule
{FedMD}&Ours w/o BAA&Ours\\
\midrule
%(FLOPs(M),Memory(GB))&
(1975.38M,14.26GB)&(947.81M,15.64GB)&(2774.19M,15.65GB)
\\
\bottomrule
\end{tabular}
\caption{Training cost analysis. A cell refers to (Flops, Memory).
}
\label{costa}
\end{table}

\begin{table*}[t]
\centering
\begin{tabular*}{\hsize}{@{}@{\extracolsep{\fill}}lccc cc c c@{}}
\toprule
\multirow{3}{*}{Method}&\multicolumn{4}{c}{Clients}&\multicolumn{3}{c}{Server}
\\\cline{2-5} \cline{6-8}&CIFAR-100&AGNEWS&\multicolumn{2}{c}{Flickr30k}&\multicolumn{3}{c}{Flickr30k}\\
\cline{2-2} \cline{3-3} \cline{4-5} \cline{6-8}
&acc@1&acc@1&i2t R@1&t2i R@1&i2t R@1&t2i R@1&rsum R@1\\
\hline
FedMD&20.63&44.37&20.93&17.75&45.50&37.32&82.82\\
FedGEMS&20.69&44.57&20.83&16.55&45.20&37.28&82.48\\
FedET&\underline{32.33}&\underline{51.03}&22.38&\underline{18.30}&45.00&\underline{37.86}&82.86\\
CreamFL&17.68&44.15&20.90&16.91&\bf{46.50}&36.74&83.24\\
FedMKD&24.58&47.11&\underline{22.65}&18.22&45.30&37.72&83.02\\
FedDFA&20.60&45.12&22.05&18.13&\underline{45.80}&37.52&\underline{83.32}\\
\midrule
FedAFD&\bf{32.58}&\bf{51.26}&\bf{35.38}&\bf{29.74}&\bf{46.50}&\bf{37.94}&\bf{84.44}\\
\bottomrule
\end{tabular*}
\caption{Impact of Discrepancy between public and private datasets. The best and second-best results are highlighted in boldface and underlined, respectively.}
\label{discrepancy}
\end{table*}

\begin{table*}
\centering
\begin{tabular*}{\hsize}{@{}@{\extracolsep{\fill}}lccc cc c c@{}}
\toprule
\multirow{3}{*}
{$\beta$}&\multicolumn{4}{c}{Clients}&\multicolumn{3}{c}{Server}
\\\cline{2-5} \cline{6-8}&CIFAR-100&AGNEWS&\multicolumn{2}{c}{Flickr30k}&\multicolumn{3}{c}{MS-COCO}\\
\cline{2-2} \cline{3-3} \cline{4-5} \cline{6-8}
&acc@1&acc@1&i2t R@1&t2i R@1&i2t R@1&t2i R@1&rsum R@1\\
\hline
0&\bf{33.56}&49.03&32.13&25.56&33.70&25.59&59.29\\
0.3&32.96&50.31&\underline{32.38}&25.50&\underline{33.90}&25.98&\underline{59.88}\\
0.5&\underline{33.18}&\bf{51.98}&\bf{32.48}&\bf{25.68}&\bf{33.98}&\bf{26.18}&\bf{60.16}\\
0.7&32.52&\underline{50.69}&32.33&\underline{25.62}&33.80&25.98&59.78\\
1.0&32.29&50.66&31.93&25.35&33.82&\underline{26.03}&59.85\\
% FedAFD($\beta=0.3$)&32.96&50.13&31.40&25.49&33.90&25.98&59.88\\
% FedAFD($\beta=1$)&32.26&50.73&31.33&25.60&33.82&26.03&59.85\\
\bottomrule
\end{tabular*}
\caption{FedAFD with varying $\beta$. The best and second-best results are highlighted in boldface and underlined, respectively.}
\label{beta}
\end{table*}

\subsection{Motivation from Domain Adaptation}
The design of the Bi-level Adversarial Alignment (BAA) module is theoretically motivated by the foundational theory of domain adaptation. The seminal work of Ben-David et al.~\cite{ben2010theory} provides a generalization bound that quantifies the expected error of a model on a target domain. Let $L_{\mathcal{D}_S}(h)$ and $L_{\mathcal{D}_T}(h)$ be the expected errors of a hypothesis on the source and target domains, respectively. The theory states:
\begin{equation}
L_{\mathcal{D}_T}(h)\leq L_{\mathcal{D}_S}(h)+ \frac{1}{2} d_{\mathcal{H}\Delta\mathcal{H}}(\mathcal{D}_S, \mathcal{D}_T) + \lambda,
\label{eq:da_bound}
\end{equation}
where $d_{\mathcal{H}\Delta\mathcal{H}}(\mathcal{D}_S, \mathcal{D}_T)$ is the $\mathcal{H}\Delta\mathcal{H}$-divergence, measuring the distribution discrepancy between the source domain $\mathcal{D}_S$ and the target domain $\mathcal{D}_T$, and $\lambda$ is the error of an ideal joint hypothesis on both domains.

We treat the challenge of representation inconsistency due to modality and task heterogeneity as a generalized federated domain adaptation problem. Specifically, the feature space learned by each client is considered the source domain $\mathcal{D}_S$, while the server's representation space is the target domain $\mathcal{D}_T$. In this view, both the modality gap and the task gap can be interpreted as manifestations of the distribution discrepancy $d_{\mathcal{H}\Delta\mathcal{H}}(\mathcal{D}_S, \mathcal{D}_T)$. The performance of the global model on its tasks is thus upper-bounded by the errors of the local models and the distribution discrepancy.

\section{Extra Experimental Results And Details}
\label{sec:a}
\subsection{Communication Cost Analysis}
The communication cost per round in FedAFD is primarily composed of two parts: 1) Server-to-Client (Download): The server broadcasts the global encoders $(\phi_g^i,\phi_g^t)$ and the global representations of the public dataset to the participating clients; 2) Client-to-Server (Upload): Clients upload their locally generated representations of the public dataset to the server. The cost is calculated based on our experimental setup where the public dataset size is $|\mathcal{P}|=10,000$ and the feature dimension $d=256$.

In the vanilla FedAFD framework, the primary communication overhead comes from the repeatedly transmitting the global encoders to all participating clients at every communication round. To address this bottleneck, we send the global encoder to clients only once every $K$ communication rounds (e.g., $K$=10), instead of every round. This approach reduces the download cost by approximately 90\%, transforming the communication complexity from $O(T\cdot M)$ to $O(\frac{T}{K}\cdot M)$ where $T$ is the total number of rounds and $M$ is the size of global encoders.

As shown in Table ~\ref{K} and Table ~\ref{communication cost}, FedAFD($K=10$) maintains competitive performance across all tasks. On the server-side MS-COCO task, it achieves a 59.88 rsum R@1, representing only a 0.28 performance drop compared to the full FedAFD (60.16), while significantly outperforming all baseline methods. More importantly, this makes our method's communication cost comparable to or better than other representation-based methods like FedET, while providing superior performance.

\subsection{Computational Cost Analysis}
We evaluate the computational overhead by measuring the average training time per communication on two NVIDIA RTX3090 GPUs.

By distributing the global encoders only once every $K$ rounds as described above, the computational overhead on clients can also be significantly reduced. Since the global encoders remain fixed during each $K$-round interval, clients can cache the features generated by the global encoder for local data. During the subsequent $(K \times E - 1)$ local training epochs, these cached features can be directly reused, substantially reducing the overall computational cost.

As shown in Table ~\ref{Computational cost}, FedAFD takes 1034 seconds per round, which is slightly longer than most other methods, but its performance is significantly improved (Table ~\ref{K}). The primary sources of overhead are the client-side bi-level adversarial training and the granularity-aware feature fusion, which involve forward passes through both local and global models. Although this results in higher communication costs per round, considering the significant performance advantages of FedAFD mentioned in the main text and the fact that it requires fewer rounds to achieve the goal, the total computational budget required to reach a high-performance target is often acceptable. Reducing the cost per round is a promising direction for future research.

Compared to FedMD and our ablation without BAA (Tab.\ref{costa}), BAA incurs only modest training overhead without additional test latency, and offers an acceptable trade-off between performance (+1.47\% gain) and cost.

\begin{figure*}[h!]
\centering
    \begin{subfigure}{0.32\linewidth}
        \centering
        \includegraphics[width=\linewidth]{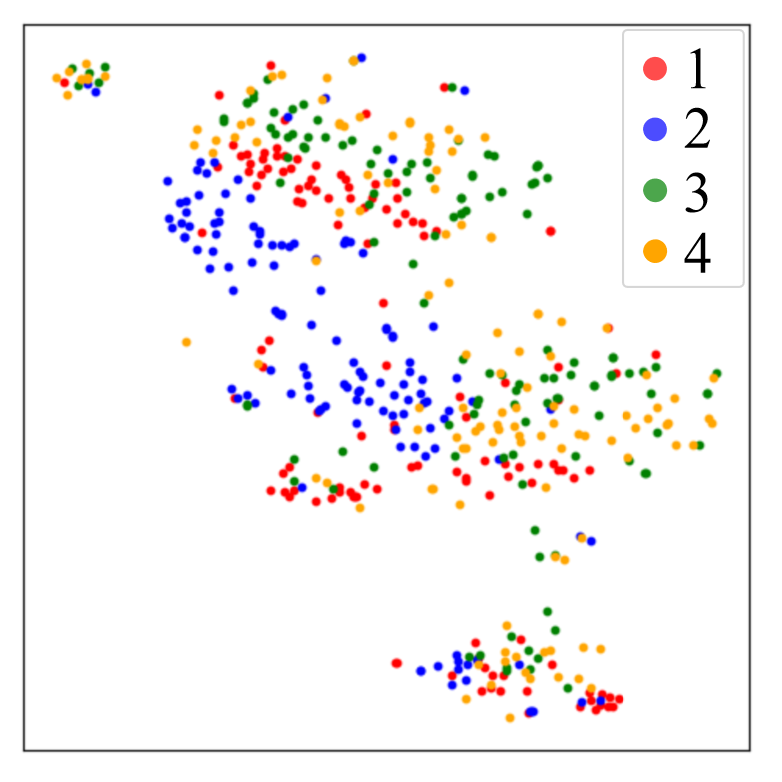}
        \caption{Locally-trained}
        \label{fig:local}
    \end{subfigure}
    \hfill
    \begin{subfigure}{0.32\linewidth}
        \centering
        \includegraphics[width=\linewidth]{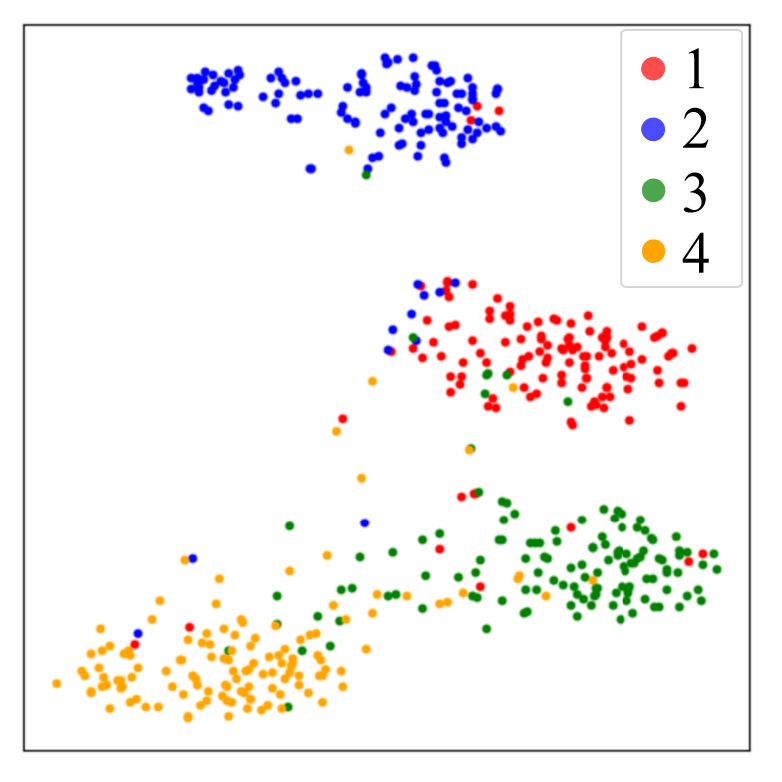}
        \caption{Fused by Category}
        \label{fig:fused}
    \end{subfigure}
    \hfill
    \begin{subfigure}{0.32\linewidth}
        \centering
        \includegraphics[width=\linewidth]{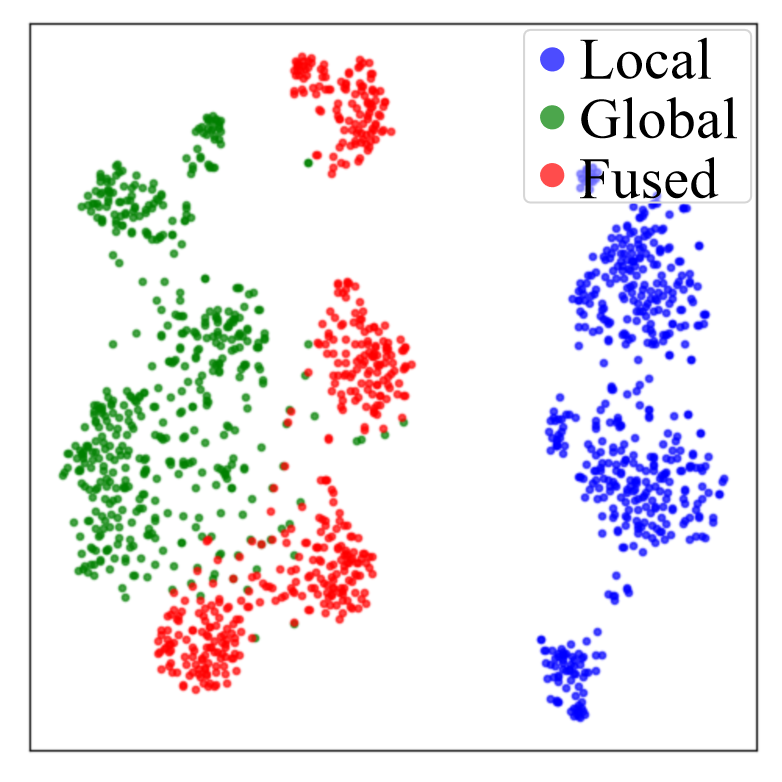}
        \caption{Entire spaces}
        \label{fig:all}
    \end{subfigure}
\caption{T-SNE visualization of different features on AGNEWS, in terms of both text category and feature types.}
\label{GFF2}
\end{figure*}

\begin{table}[t]
\centering
\begin{tabular}{lccc}
\toprule
Client Composition & i2t R@1 & t2i R@1 & rsum R@1 \\
\hline
FedAFD & 33.78 & 26.02 & 59.80 \\
\midrule
Fewer Image & 33.40 & 25.88 & 59.28 \\
Fewer Text & 33.38 & 25.95 & 59.33 \\
Fewer Multimodal & 32.96 & 25.89 & 58.85 \\
\bottomrule
\end{tabular}
\caption{Impact of client composition on server performance.}
\label{tab:client_composition}
\end{table}

\begin{table}[t]
\centering
\footnotesize
\begin{tabular*}{\hsize}{@{}@{\extracolsep{\fill}}lccc c@{}}
\toprule
\multirow{3}{*}{Method}&\multicolumn{3}{c}{Clients}&\multicolumn{1}{c}{Server}
\\\cline{2-4} \cline{5-5}&CIFAR-100&AGNEWS&\multicolumn{1}{c}{Flickr30k}&\multicolumn{1}{c}{MS-COCO*}\\
\cline{2-2} \cline{3-3} \cline{4-4} \cline{5-5}
&acc@1&acc@1&rsum R@1&rsum R@1\\
\hline
LOCAL&28.07&48.35&40.77&55.97\\
FedAFD&\textbf{32.03}&\textbf{50.90}&\textbf{58.27}&\textbf{58.88}\\
\bottomrule
\end{tabular*}
\caption{OOD test with semantical-irrelevant subset MS-COCO*.}
\label{ood}
\end{table}

\begin{table}[t]
\centering
\footnotesize
\begin{tabular*}{\hsize}{@{}@{\extracolsep{\fill}}lccc c@{}}
\toprule
\multirow{3}{*}{Method}&\multicolumn{3}{c}{Clients}&\multicolumn{1}{c}{Server}
\\\cline{2-4} \cline{5-5}&CIFAR-100&AGNEWS&\multicolumn{1}{c}{Flickr30k}&\multicolumn{1}{c}{MS-COCO}\\
\cline{2-2} \cline{3-3} \cline{4-4} \cline{5-5}
&acc@1&acc@1&rsum R@1&rsum R@1\\
\hline
Averaging&32.21&50.20&56.97&59.56\\
Aggr-MM&33.06&51.68&58.09&59.91\\
SED&\textbf{33.18}&\textbf{51.98}&\textbf{58.16}&\textbf{60.16}\\
\bottomrule
\end{tabular*}
\caption{Performance under varied
server aggregation methods.}
\label{mmonly}
\end{table}

\subsection{Impact of Discrepancy between public and private datasets}
A key question in federated learning with a public dataset is how does the discrepancy between the public data and the clients' private data affect performance. To investigate this, we designed a controlled experiment in which we replaced the server's public MS-COCO dataset with 10K Flickr30k samples, which are aligned with the multimodal clients' private data. This setup minimizes the domain gap between public and private multimodal datasets.

As shown in Table~\ref{discrepancy}, FedAFD still achieves the best performance among all methods. There is no significant change in performance on the unimodal client compared to using MS-COCO as the public dataset. However, performance on multimodal clients and servers showed significant improvements, indicating that the smaller the difference between public and private data, the better the performance.

In a new extreme OOD setting (see Tab.\ref{ood}), removing all client-related categories from MS-COCO, FedAFD still performs the best, demonstrating robustness across OOD levels.

\subsection{Effect of Alignment Loss Weight $\beta$}
We vary the alignment loss weight $\beta$ in the BAA module to investigate its impact on the trade-off between representation alignment and task performance. Specifically, we evaluate $\beta \in \{0, 0.3, 0.5, 0.7, 1.0\}$ under the Non-IID setting. As shown in Table~\ref{beta}, moderate values (e.g., $\beta=0.5$) yield the best performance across clients and the server, confirming that appropriate adversarial alignment helps bridge the modality and task gaps without overwhelming task learning. Overly high or low values of $\beta$ adversely affect both local adaptation and global representation alignment.

\subsection{Impact of Client Composition}
To investigate how the composition of client modalities affects global model performance, we conduct sensitivity analysis by systematically reducing the number of clients in each modality. The original FedAFD configuration uses 3 image clients, 3 text clients, and 4 multimodal clients. We compare three reduced scenarios:\\
1 Fewer Image: 1 image, 3 text, 4 multimodal clients.\\
2) Fewer Text: 3 image, 1 text, 4 multimodal clients.\\
3) Fewer Multimodal: 3 image, 3 text, 2 multimodal clients.

The performance on the server's MS-COCO retrieval task is summarized in Table ~\ref{tab:client_composition}. It can be observed that reducing clients from any modality impairs server performance, and reducing multimodal clients results in a greater decrease than unimodal clients. This suggests that for the server's cross-modal retrieval tasks, multimodal clients contribute more knowledge than unimodal clients.

\subsection{Visualization of GFF Module}
To further validate the impact of the GFF module on client-side feature representation, we conduct a comparative t-SNE visualization analysis using the AGNEWS dataset. As shown in Fig.~\ref{GFF2}, we visualize features from the four classes under three settings: using the local encoder only (``Local''), using the global encoder (``Global''), and using the GFF-based fusion (``Fused''). Fig.~\ref{GFF2}(a) and Fig.~\ref{GFF2}(b) show class-wise distributions, while Fig.~\ref{GFF2}(c) presents an overall comparison.
The results reveal that the fused features exhibit more precise inter-class boundaries than ``Local'', demonstrating that GFF effectively improves local feature discriminability by integrating global semantics. This confirms that FedAFD balances global knowledge integration with client-specific task optimization.

Local features, focused on specific classification tasks, capture partial information and thus appear noisier. Global features, distilled from multiple clients, incorporate broader knowledge and retain local task separability (see Fig.\ref{fig:gfeature}). Fusing them via GFF produces the most discriminative, least noisy clusters.

\begin{figure}[t]
\centering
\includegraphics[width=0.8\linewidth]{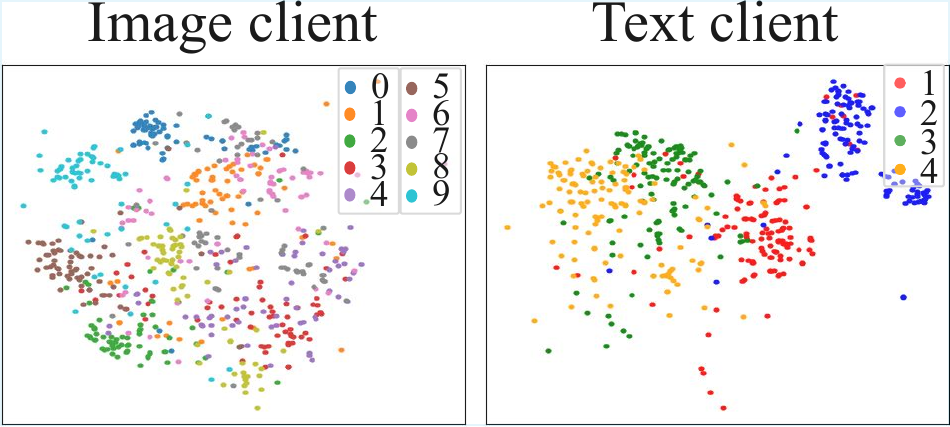}
\caption{Per-category global features.}
\label{fig:gfeature}
\end{figure}

\begin{figure}[t]
\centering
\includegraphics[width=\columnwidth]{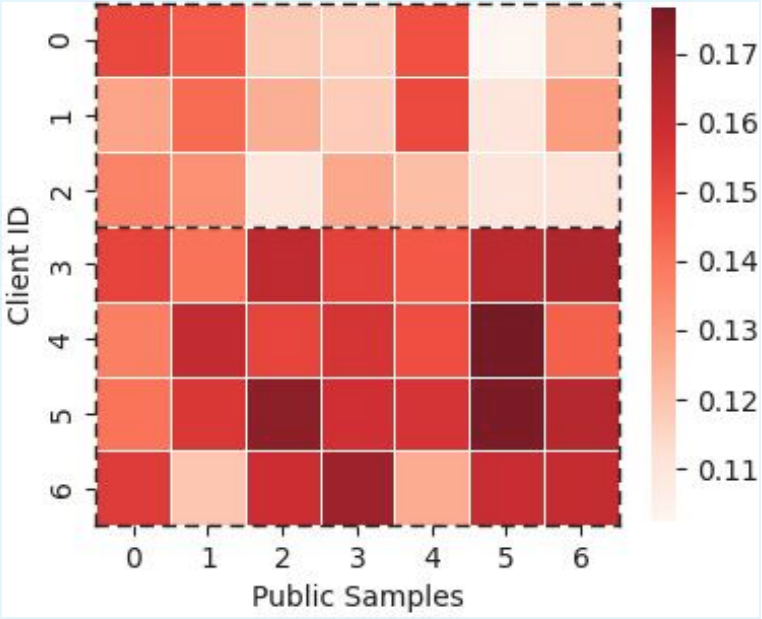}
\caption{Aggregation weight heatmap of image clients}
\label{heatmap}
\end{figure}

\subsection{Ablation of SED Module}
An ablation replacing SED with server aggregation using only multimodal clients (``Aggr-MM'') shows that SED outperforms both naive averaging and retrieval-only aggregation (see Tab.\ref{mmonly}). The heatmap Fig.~\ref{heatmap} illustrates the final aggregation weights assigned to clients with image modality across seven random public samples. Rows Client ID 0, 1 and 2 correspond to unimodal image clients, while the rest correspond to multimodal clients. Each column represents the client-wise weight distribution for a specific public sample. It can be observed that multimodal clients generally receive higher weights compared to unimodal clients. This phenomenon can be attributed to the fact that multimodal clients can access and integrate both image and text modalities and their extracted features are naturally more aligned with the server’s modality reference features. Consequently, they achieve higher similarity scores during the aggregation process. However, unimodal clients may also receive relatively high weights on certain samples, suggesting that they can also contribute to the aggregation process.
